# Supplementary material for: Interface-Induced Conservation of Momentum Leads to Chiral-Induced Spin Selectivity
Source: arXiv:2111.14770 source file (2021-11-29)

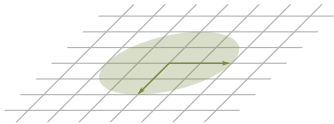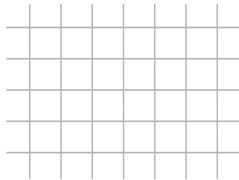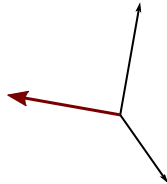

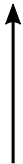

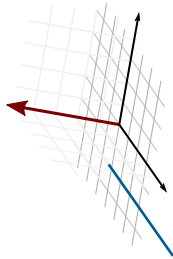

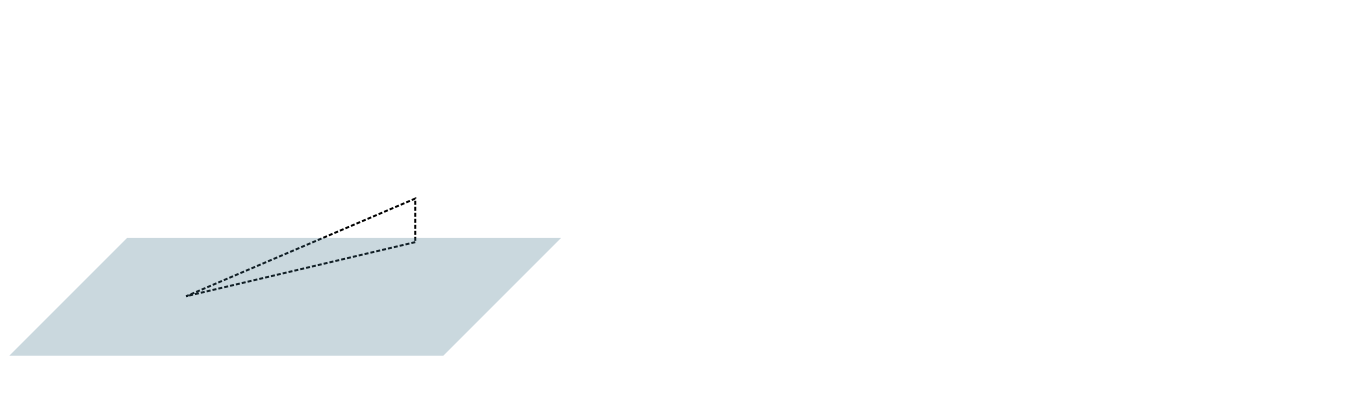

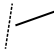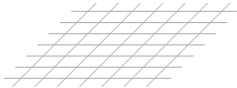

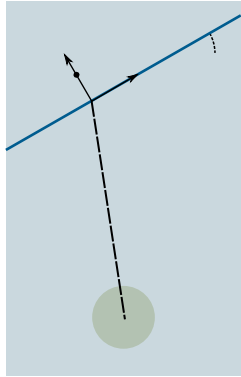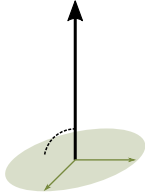

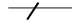

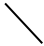



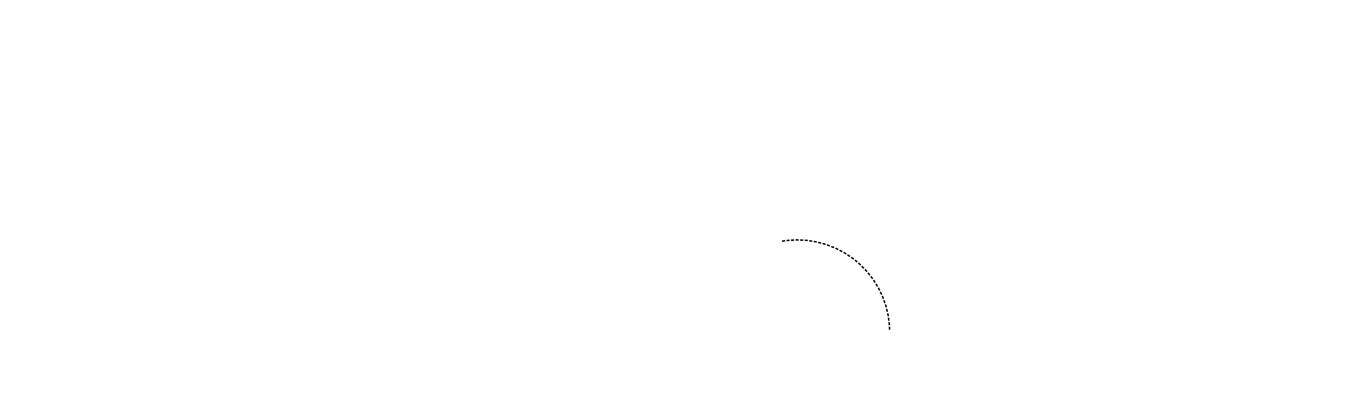

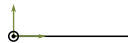

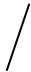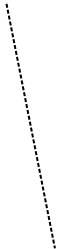

}

1

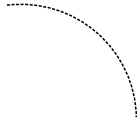

Supplement: Supplementary file 2 [file drawing_sidebyside.pdf]
